# Supplementary material for: Lattice QCD for Cosmology
Source: arXiv:1606.07494 source file (2016-06-27)
Supplement: Supplementary file 1 [file som_eos_old.tex]

\section{Equation of state of the Standard Model}
\label{se:som_eos}

It has been a longstanding challenge to determine the pressure,
energy density, and the number of effective degrees of freedom as a function of
the temperature from first principles.
This is the equation of state of the universe. Cosmology
requires this information over many orders of magnitude,
ranging from beyond the electroweak scale down to the decoupling
of matter on the $eV$ scale \cite{Srednicki:1988ce,Hindmarsh:2005ix}.
The equilibrium equation of state, that assumes all particles to be
in thermal equilibrium, is relevant down to a temperature of approximately
$1~\mathrm{MeV}$ when neutrinos decouple from the heatbath.

As the Universe covers this broad temperature range it passes though several
epochs, each with a different dominant interaction. We restrict our study here
to the Standard Model of particle physics.
At the high end of the temperature range of interest there is the
electroweak phase transition at $159.5\pm1.5$~GeV temperature
\cite{Onofrio:2015mpa}.  The equation of state of
the electroweak transition has been worked out in
Refs.~\cite{Laine:2006cp,Laine:2013raa,Laine:2015kra} with the intent to
provide a description for the entire Standard Model. For this reason the
contribution from all other degrees of freedom (i.e. up to the bottom quark)
had to be estimated. While the photon, neutrinos and leptons can easily be
described as practically free particles, the QCD part requires a
non-perturbative approach. This was not available by the time
Refs.~\cite{Laine:2006cp,Laine:2013raa} were published. 

In this paper we add the last missing piece to the cosmological equation of
state: the QCD contribution. In this section we describe our method to obtain
the QCD equation of state up to 1 GeV temperature scale.  Then we will be in
the position to compare the result to the standard and HTL perturbation theory.
This is a very important step, since this validates the perturbative 
approach that will be used throughout the electroweak epoch. We also work out
the bottom contribution in a simple but efficient approximation.
Then we combine the elements of the Standard Model and
present the number of effective degrees of freedom from the energy
density and entropy ($g_{\rho}(T)$ and $g_{s}(T)$) in the full range.


\subsection{The 2+1+1 flavor QCD equation of state }

For 2+1 dynamical flavors with physical quark masses we calculated
the equation of state in Ref.~\cite{Borsanyi:2010cj,Borsanyi:2013bia}.
This result was later confirmed in Ref.~\cite{Bazavov:2014pvz}.
The effect of the charm quark has been estimated by several authors
using perturbation theory \cite{Laine:2006cp}, or partially quenched
lattice simulations \cite{Cheng:2007wu,Levkova:2009gq}, or from
simulations with four non-degenerate quarks, but unphysical masses
\cite{Burger:2013hia,Bazavov:2013pra}.
However, the final results must come from a dynamical simulation where all
quark masses assume their physical values \cite{Borsanyi:2012vn}.

We meet this challenge by using a 2+1+1 flavor staggered action (with 4 levels
of stout smearing), that we have introduced in Section \ref{se:som_zero}. 
The action parameters, the bare quark masses and the tuning procedure, as well
as the lattice geometries and  statistics have been given in detail in
Ref.~\cite{Bellwied:2015lba}.

We calculate the trace anomaly ($I=\epsilon-3p$) for each finite temperature
lattice ensemble.

\begin{equation}
\frac{I(T)}{T^4}=\frac{\varepsilon-3p}{T^4}= N_t^4
R_\beta
\left[
\frac{\partial}{\partial \beta}
+\sum_f R_{m_f} am_f \frac{\partial}{\partial am_f}
\right]\frac{\log Z[am_u,am_d,am_s,...]}{N_t N_s^3}
\label{eq:traceaexpression}
\end{equation}
with
\begin{equation}
R_\beta = - \frac{d \beta}{d\log a}\qquad\mathrm{and}\qquad
R_{m_f}= \frac{d\log m_f}{d\beta}, \quad f=u,d,s,\dots\,.
\end{equation}
The derivative of $\log~Z$ with respect to the gauge coupling 
$\beta$ and the mass (in lattice units) $am$ are easily accessible
observables on the lattice: the gauge action $S_g$ and the chiral
condensate, respectively.

The running of the coupling and the mass is universal at low
orders of perturbation theory: e.g. for QCD with $N_f$ flavors we have 
$R_\beta=12b_0+72b_1/\beta+\mathcal{O}(\beta^{-2})$ with
$b_0=(33-2N_f)/48\pi^2$ and $b_1=(306-38N_f)/768\pi^2$. However, in the phenomenologically
relevant range of parameters and accessible lattice spacings one has
to calculate $R_\beta(\beta)$ and the $R_m(\beta)$ functions
non-perturbatively with zero temperature simulations along with the
determination of the line of constant physics. Since $R_\beta$ appears
as a factor in front of the final result, the systematics of the scale
setting directly distorts the trace anomaly. For this reason we
calculate $R_\beta$ both from the $w_0$ and the $f_\pi$-based scale
setting and include the difference in the systematical error estimate.

There is an additive, temperature independent divergence in the trace
anomaly. In the standard procedure, that we also followed in
Ref.~\cite{Borsanyi:2010cj} each finite temperature simulation is
accompanied by a zero temperature ensemble. The trace anomaly is then 
calculated on both sets of configurations, their difference is the physical
result. This defines a renormalization scheme where the zero temperature
pressure and energy density are zero.

This strategy is bound to fail at higher temperatures. In lattice thermodynamics
the temperature is set by the lattice spacing ($a$) and the temporal resolution $N_t$
as $T=1/aN_t$. $N_t$ cannot be chosen below 6 or 8 if a near-continuum behaviour
is desired. Thus, high temperatures can only be achieved with very fine lattices.
As the lattice spacing is reduced, the autocorrelation times for
zero temperature simulations raise, and the costs of these simulations explode beyond
feasibility. Notice, however, that the renormalization constant is accessible
not only from zero temperature simulations, but from any finite temperature
data point that was taken with the same lattice spacing (i.e. same gauge
coupling) and some bare masses. 

In our approach we generate a renormalization ensemble for each finite
temperature ensemble at exactly half temperature with the same physical volume
and matching bare parameters. The trace anomaly difference is then divergence-free.
We have tested this idea in the quark-less theory in
Refs.~\cite{Endrodi:2007tq,Borsanyi:2012ve}.

Thus we determine the quantity $[I(T)-I(T/2)]/T^4$ in the temperature
range 250\dots 1000~MeV for four resolutions $N_t=6,8,10$~and~12. The volumes
are selected such that $LT_c\gtrsim2$. In Fig.~\ref{fig:trah} we show this
subtracted trace anomaly and its continuum limit. 

\begin{figure}[ht]
\centerline{\includegraphics[width=3in]{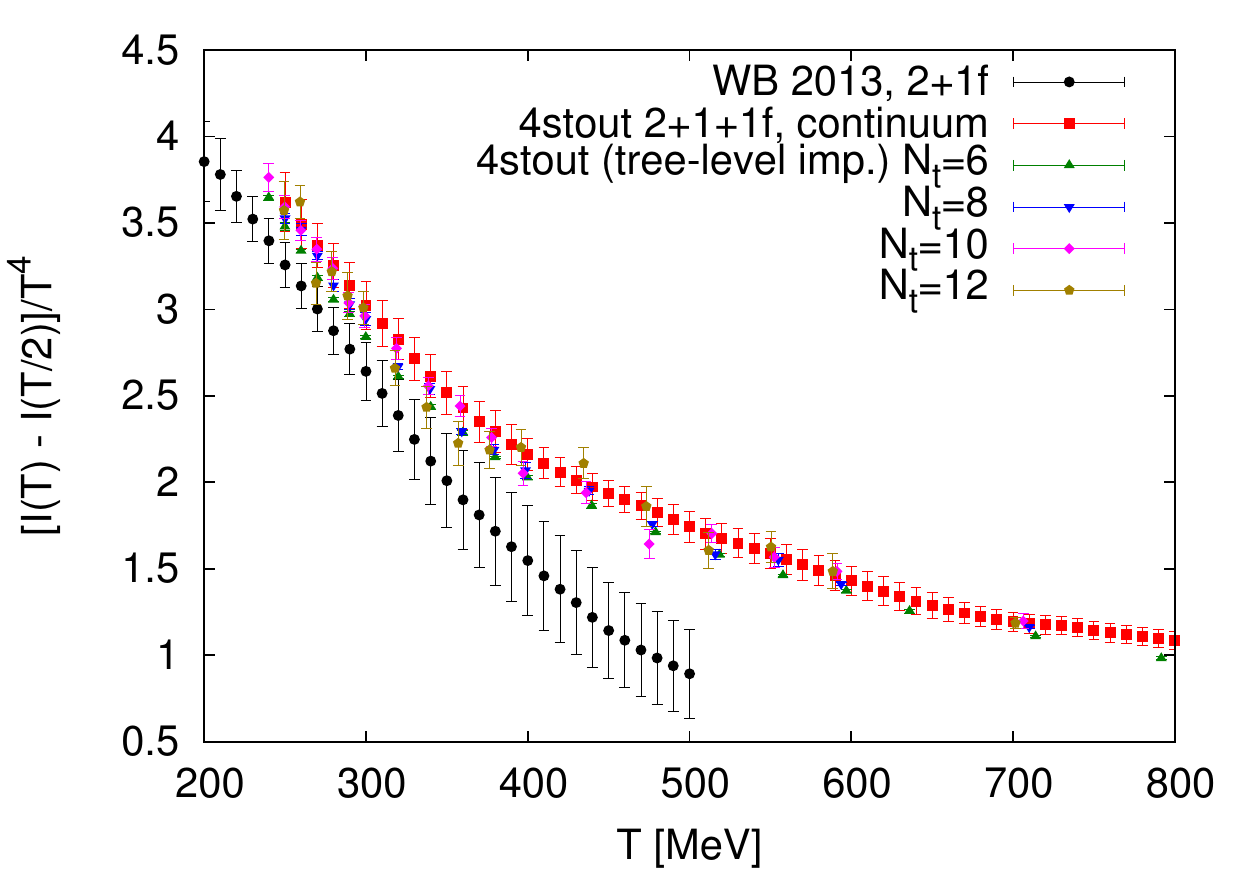}}
\caption{
The subtracted trace anomaly in the 2+1+1 and 2+1 flavor theories. We also
show the individual lattice resolutions $(N_t=6\dots12)$ that contribute
to the continuum limit.
\label{fig:trah}
}
\end{figure}

For obtaining the continuum limit we used the same procedure as in
Ref.~\cite{Bellwied:2015lba}: we interpolated the lattice data in temperature
and then we performed a continuum extrapolation in $1/N_t^2$ temperature by
temperature.  The error bars in Fig.~\ref{fig:trah} combine the statistical and
systematical errors, the latter we estimate by varying the scale setting
prescription ($w_0$-based or $f_\pi$-based scale setting), the observable
(subtracted trace anomaly or its reciprocal), the interpolation, and whether or
not we use a tree-level improvement prior to the continuum extrapolation
\cite{Borsanyi:2010cj}.

Then we use the already established 2+1 flavor equation of state to calculate
$I(T)/T^4$ from the continuum limit of $[I(T)-I(T/2)]/T^4$ using the formula:
\begin{equation}
\frac{I(T)}{T^4}=
\sum_{k=0}^{n-1}\left.\frac{I\left(T/2^k\right)-I\left(T/2^{k+1}\right)}{\left(T/2^k\right)^4}\right|_{N_f=2+1+1}
+
\left.\frac{I\left(T/2^n\right)}{\left(T/2^n\right)^4}\right|_{N_f=2+1}\,,
\end{equation}
where $n$ is the smallest non-negative integer with $T/2^n <250~\mathrm{MeV}$.

The temperature integral of $I(T)/T^5$ gives the normalized pressure
$p(T)/T^4$.  The energy density ($\epsilon$) and entropy density ($s$) are
obtained from thermodynamical relations: $\epsilon=I+3p$ and $sT = \epsilon+p$,
respectively.

In Ref.~\cite{Borsanyi:2013bia} we have given a simple parametrization for the
2+1 flavor equation of state. Here we present a new version that covers the
100-1000~MeV temperature range and is consistent with the 2+1+1 lattice data 
(including the QCD contribution only).
\begin{equation}
\frac{I(T)}{T^4} = \exp(-h_1/t-h_2/t^2)\cdot\left( h_0 + f_0 \frac{ \tanh(f_1\cdot t+f_2)+1}{1+g_1\cdot t + g_2 \cdot
t^2} \right),
\label{eq:param211}
\end{equation}
with $t=T/200~\mathrm{MeV}$. The parameters are given in Table.~\ref{tab:coeffs}.



\begin{table}
\begin{center}
\begin{tabular}{|c||c|c|c|c|c|c|c|c|}
\hline
&$h_0$&$h_1$&$h_2$&$f_0$&$f_1$&$f_2$&$g_1$&$g_2$\\
\hline
\textbf{2+1+1 flavors} & 0.1396 & -0.180 & 0.035 & 3.34 & 5.74 & -4.43 & 0.756 &0.185 \\
\textbf{2+1 flavors~\cite{Borsanyi:2013bia}}& 0.1396 & -0.180 & 0.035 & 1.05 & 6.39 & -4.72 & -0.92 &0.57 \\
\hline
\end{tabular}
\end{center}
\caption{\label{tab:coeffs}
Constants for our parametrization of the trace anomaly in Eq.~(\ref{eq:param211}).
}
\end{table}


\subsection{Comparison to previous estimates}

Plotting the $p/T^4$ (which is the normalized free energy density),
we can compare the final result to other approaches. At low temperatures
the Hadron Resonance Gas model (using the 2014 PDG spectrum) gives a fair
description of lattice data. This was already observed in
Ref.~\cite{Borsanyi:2013bia}. At high temperature recent progress in Hard
Thermal Loop perturbation theory has provided for a
next-to-next-to-leading-order result for the free energy, which is in
good agreement with our data both for the 2+1 theory \cite{Andersen:2010wu}
and also for the 2+1+1 flavor theory for high enough temperatures where the charm
mass is small in comparison to $\pi T$.
We show the 2+1+1 flavor result in Fig.~\ref{fig:pressure}.

\begin{figure}[ht]
\centerline{\includegraphics[width=2.5in]{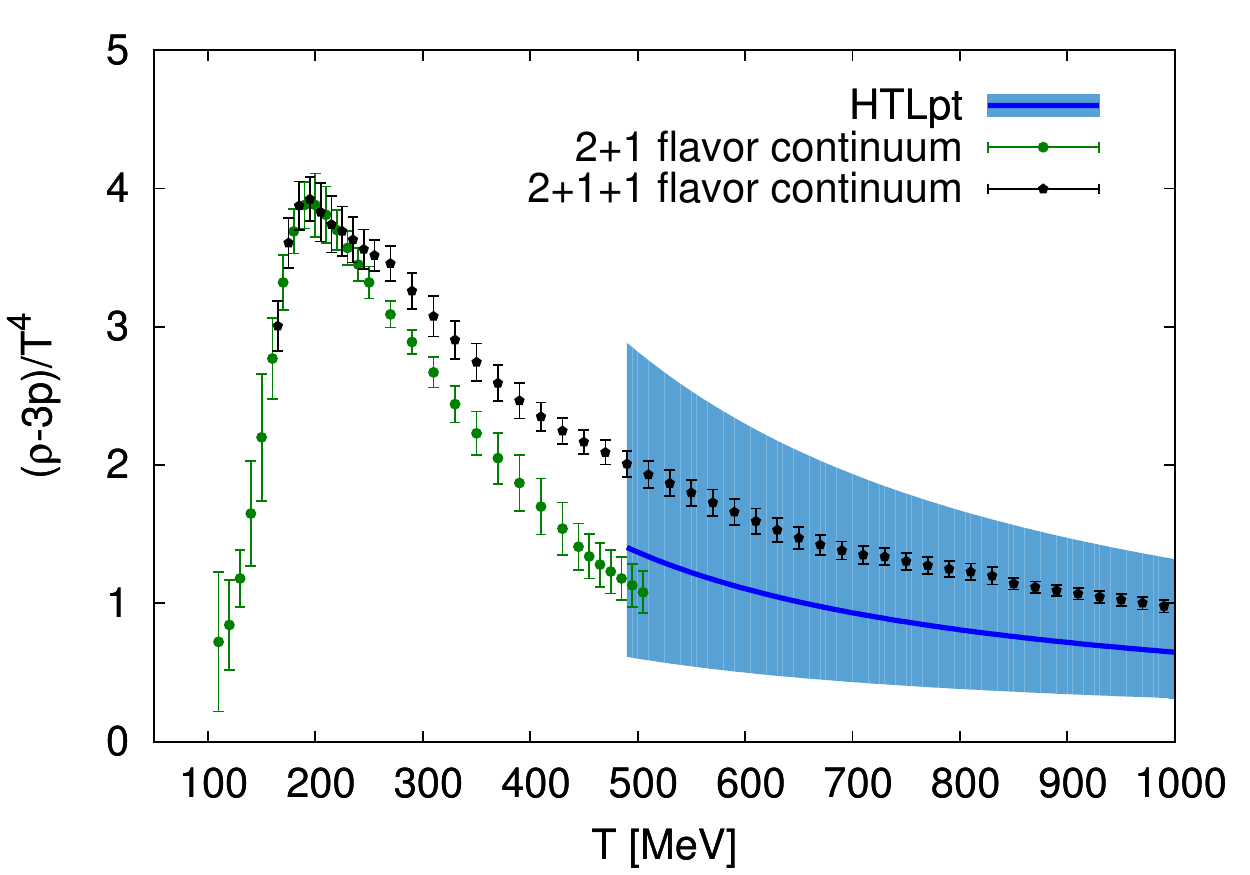}\hspace{1cm}
\includegraphics[width=2.5in]{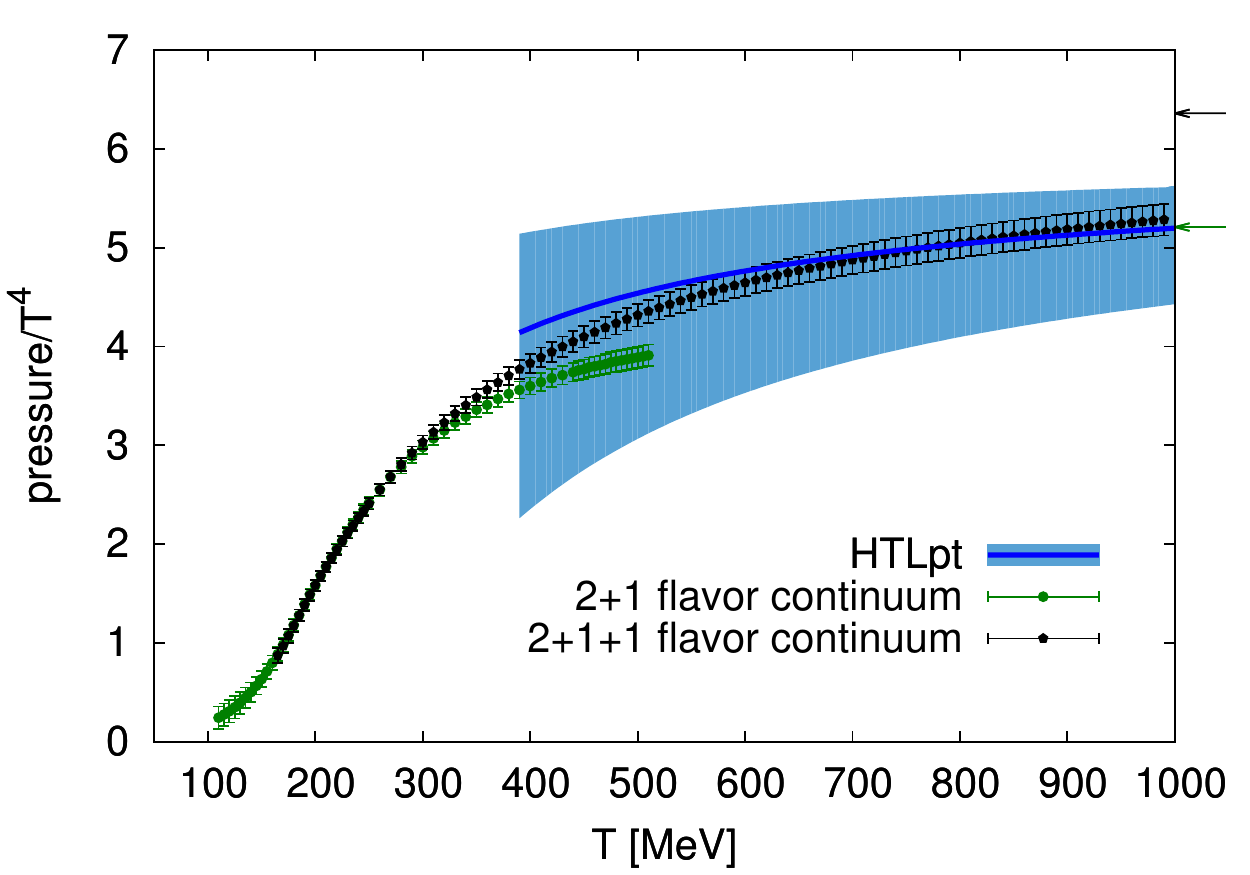}}
\caption{
The QCD trace anomaly pressure in the 2+1+1 and 2+1 flavor theories. We give the
Hadron Resonance Gas prediction at low temperatures
as well as the four flavor NNLO Hard Thermal Loop result at high temperatures
\cite{Andersen:2010wu}. The red lines represent or preferred parametrization
Eq.~(\ref{eq:param211}).
\label{fig:pressure}
}
\end{figure}

We also show a comparison to the results of conventional perturbation theory
with four massless quarks in Fig.~\ref{fig:pcmp}. The completely known fifth
order \cite{Zhai:1995ac} is already close to the lattice data. The difference
can mostly be attributed to the so far ignored mass of the charm quark.

\begin{figure}[ht]
\begin{center}
\includegraphics[width=4in]{figs/eos/pcmp}
\end{center}
\caption{\label{fig:pcmp}
The QCD pressure for 2+1+1 flavors together with the estimate by
Laine\&Schr\"oder \cite{Laine:2006cp}  and the various orders of conventional
perturbation theory.
}
\end{figure}

The quark mass threshold for the charm quark entering the QCD equation of state
has already been estimated by Laine and Schr\"oder in Ref.~\cite{Laine:2006cp}.
There the effect of a heavy quark was calculated to a low order of perturbation theory.
This effect was expressed as a pressure ratio between the 3+1 and 3 flavor
theories, which was translated to the final result using the 3 flavor result.
By the time of that paper the lattice result for the QCD equation of state was
not yet available, but perturbative results have already been in an advanced state.
For zero masses, which is a reasonable assumption up to $N_f=3$ above
the QCD transition, the perturbative equation of state is known to $g^6\log g$
order
\cite{Kajantie:2002wa}. The $g^6$ order already contains non-perturbative contributions.
Through dimensional reduction and the
lattice simulation of the resulting 3-dimensional effective theory even that
was calculated in the quenched theory, though a comparison to lattice data was
not encouraging \cite{Hietanen:2008tv}

Despite the known difficulties of perturbation theory the estimate of
Ref.~\cite{Laine:2006cp} is very close to our lattice result if we plot
the ratio of the pressure with and without the charm quark included. 
We show our lattice data together with the perturbative
estimate in Fig.~\ref{fig:charm_effect}. 


\begin{figure}[ht]
\begin{center}
%\includegraphics[width=3in,angle=270]{charm_effect}
\includegraphics[width=4in]{figs/eos/ratio}
\end{center}
\caption{\label{fig:charm_effect}
The ratio of the pressure between 2+1+1 flavor and 2+1 flavor theories from our 
lattice simulations. We also show two perturbative estimates of the ratio of the pressures in
the $3+1$ and $3$ flavour theories: The tree-level ($\mathcal{O}(g^0)$) estimate (see text),
and the $\mathcal{O}(g^2)$ estimate of Ref.~\cite{Laine:2006cp}. Both of these estimates 
show an excellent agreement with the lattice data.
}
\end{figure}

While the magnitude of either of the 2+1 or 2+1+1 flavor results does not match
with the estimate in Ref.~\cite{Laine:2006cp}, the comparison in
Fig.~\ref{fig:charm_effect} shows agreement with the data.

The tree-level charm correction 
\begin{equation}
\frac{p^{(3+1)}(T)}{p^{(3)}(T)}=\frac{SB(3) + F_Q(m_c/T)}{SB(3)}\,
\label{eq:charmcorr3}
\end{equation}
where $SB(3)$ and $SB(4)$ the Stefan Boltzmann limit of the 3 and
4 flavor theories, respectively, and $F_Q(m/T) T^4$ is the free energy of a free
quark field with mass $m$.

The $g^2$ order in the ratio of Fig.~\ref{fig:charm_effect} is a relevant
correction near $2 - 3 T_c^{QCD}$ temperature. The $2T_c$ the difference
between the two approximations is $3\%$. The difference reduces to 0.2\% at
1~GeV up to which point we have lattice data.

\subsection{QCD in the perturbative regime}

In order to improve on the perturbative result still further we
introduce the tree-level version of the 3+1 flavor perturbative
equation of state based on the four flavor theory. We introduce
the tree-level quark mass thresholds as
\begin{equation}
p^{(3+1)}(T) = p^{(4)}(T) \frac{SB(3) + F_Q(m_c/T)}{SB(4)}\,
\label{eq:charmcorr}
\end{equation}
The error of not using the $g^2$ order
is about 0.2\% of the total QCD contribution at 1 GeV. 
In this strategy we only assume the convergence of the 4 flavor
perturbation theory at 1 GeV. 
This is a much milder
assumption than requiring the perturbative behaviour for $N_f=0$ or for
$N_f=3$ at the temperatures where data are available.
Using $\Lambda_{\overline{MS}}=265$~MeV we calculated the $g^5$ order result 
with the charm mass correction in Eq.~\ref{eq:charmcorr},
which is in good agreement with the data.

For completeness we also determine the $g^6$ order. The coefficient
of the $g^6$ order is not known analytically, but the missing term, $q_c$
(following the notation of Ref.~\cite{Kajantie:2002wa}) can be
fitted against lattice data.
The $g^6$ order result describes our pressure data at 1 GeV
within errors if $-3500 < q_c < -2900$, for the trace anomaly we have $-3100 <
q_c < -2800$. We show the fitted curves in Fig.~\ref{fig:withmass}.

\begin{figure}[ht]
\centerline{
\includegraphics[width=2.5in]{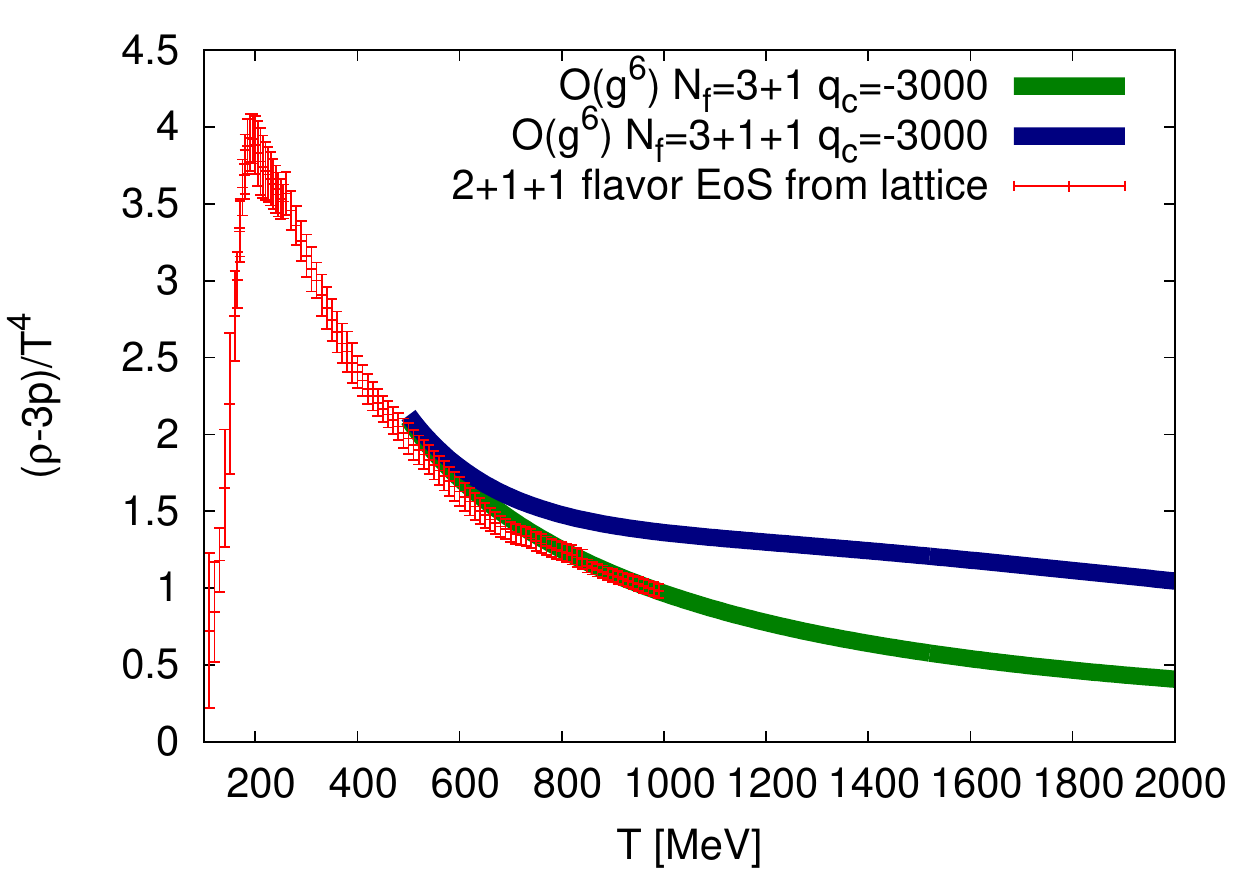}
\includegraphics[width=2.5in]{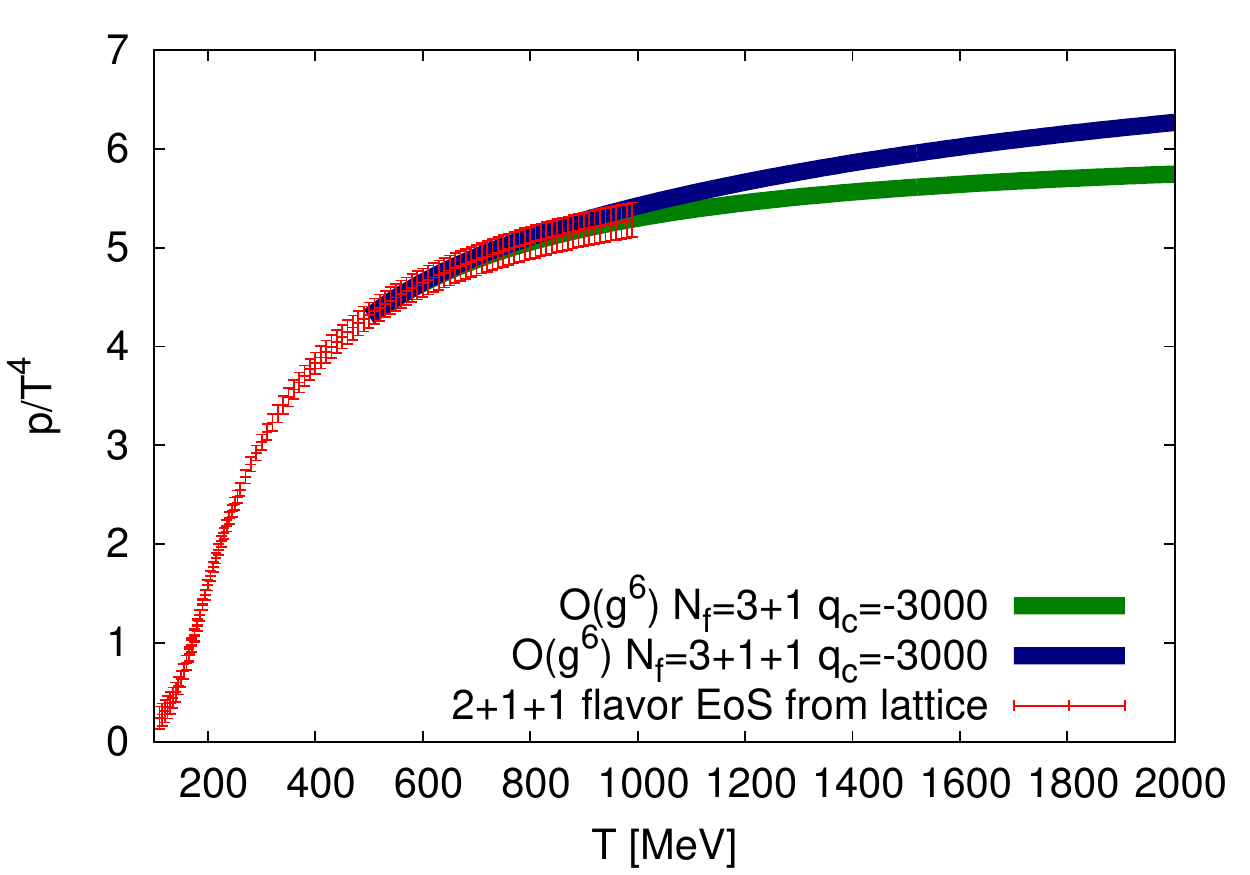}
}
\caption{\label{fig:withmass}
The lattice result for the 2+1+1 flavor QCD pressure together with the fitted
value of the $g^6$ order in Ref.~\cite{Kajantie:2002wa}. We included
the charm mass at tree-level. Using the same fitted coefficient we also
calculated the effect of the bottom quark with a similar method.
The blue curve shows the bottom threshold.
}

\end{figure}


Our lattice simulation is limited to 2+1+1 flavors, although near 1~GeV
the bottom quark is also expected to start playing a significant role.
The tree-level correction for the bottom quark reads
\begin{equation}
p^{(4+1)}(T) = p^{(4)}(T) \frac{SB(4) + F_Q(m_b/T)}{SB(4)}\,
\label{eq:bottomcorr}
\end{equation}
where $m_b$ is the bottom mass. Eq.~(\ref{eq:bottomcorr}) works
beyond the bottom threshold, too, since the ratio of the perturbative
massless 4 and 5 flavor pressures is, to a very good approximation, equal
to the ratio of the Stefan-Boltzmann limits. Comparing the free energy
up to $g^5$ order this statement holds to 0.3\% accuracy in the entire
relevant temperature range.

In Fig.~\ref{fig:withmass} we show
the 3+1+1 flavor result as well, using both factors 
(\ref{eq:charmcorr}) and (\ref{eq:bottomcorr}).

Since the massless four flavor perturbative result is used as a starting point
for both heavy quarks we have a fair approximation between 1 and 10 GeV
with one analytical formula.  The error on the lattice data propagates through
the $q_c$ parameter into the perturbative result, thus a smooth continuation
from the lattice data is possible (see Fig.~\ref{fig:gqcd}).


\subsection{The Standard Model}

Now we are in the position to construct an equation of state that gives
a fair description over the entire temperature range of the Standard Model.

In particular, we compute the effective number of degrees of freedom. These are defined
by the energy density or the entropy normalized to the Stefan-Boltzmann limit of
a single scalar field:
\begin{equation}
g_{\rho}(T)=\epsilon(T)\frac{30}{\pi^2T^4}\,,\qquad
g_{s}(T)=s(T) \frac{45}{2\pi^2T^3}\,.
\end{equation}

The final result is the combination of the following contributions:

\textit{a) Photons and neutrinos.}\\
We treat these light particles as interaction-free particles, assuming three
generations, of left-handed neutrinos. In this paper we work out the equilibrium
equation of state, here the neutrinos are not decoupled but give a trivial
contribution of $p_\nu/T^4 = \frac{7}{8} \cdot 2 \cdot 3 \cdot \pi^2/90$, for the photons
we have $p_\gamma/T^4 = \pi^2/45$.

\textit{b) Leptons}\\
We sum the free enegy of the non-interacting leptons with the formula
\begin{equation}
p/T^4 = \frac{1}{2\pi^2} \sum_i g_i \left(\frac{m_i}{T}\right)^2 \sum_{k=1}^{\infty} \frac{(-1)^k}{k^2} K_2\left(\frac{mk}{T}\right)\,,
\label{eq:fermionsum}
\end{equation}
where $K_2$ is a modified Bessel function of the second kind, and $g_i$ is the 
spin degeneracy factor, $g_i=4$ for lepton type. The right hand side of Eq.~(\ref{eq:fermionsum}) with $g_i=12$ gives the free quark contribution $F_Q(m_i/T)$ already introduced
in Eq.~(\ref{eq:charmcorr3}).

\textit{c) Light hadrons}\\
In Refs.~\cite{Borsanyi:2013bia,Bellwied:2015lba} we have tested the Hadron Gas
Model's prediction in detail. Here we use this model's prediction up to 120~MeV
temperature. From that point we switch over to the lattice result.

\textit{d) QCD}\\
We have continuum extrapolated lattice results for the equation of state up to 1~GeV
temperature. We have found these as a combination of 2+1 and 2+1+1 flavor simulations.
%Their small difference at the matching point of 250~MeV is added to the systematic
%error in quadrature.
In Fig.~\ref{fig:withmass} we have shown that the sixth order 
(highest order with one fitted coefficient) perturbative result gives a good
description of both the pressure and the trace anomaly.
Thus, we simply continue with this order. A typical estimate of the theoretical
uncertainties comes from the sensitivity of the results to the variation of the
renormalization scale between $\mu = \pi T \dots 4 \pi T$. At 1 GeV this gives a much
larger error than our lattice error, and would not faithfully represent the
available information. Instead, we put an error on the fitted coefficient 
$q_c$ and represent the perturbative result with an error band corresponding to
the range $ -3500 < q_c < -2800 $. This way the lattice data has put as strong
constraint on the perturbative estimate.

\begin{figure}[ht]
\begin{center}
\includegraphics[width=3in]{figs/eos/gqcd}
\end{center}
\caption{
\label{fig:gqcd}
The number of effective degrees of freedom $g(T)$ in the QCD epoch
from our lattice data, continued with the $g^6$ order perturbative result.
The earlier estimate \cite{Laine:2006cp} is shown for comparison.
}
\end{figure}

We show our result for $g_{\rho}(T)$ in Fig.~\ref{fig:gqcd} together with \cite{Laine:2006cp}
for comparison. The earlier estimate, which was produced without reliable
input, is close to our lattice-based result. The most significant deviation
is between 1 and $2T_C^{QCD}$, where the non-perturbative physics is 
dominant and one cannot rely on phenomenological models, like the HRG.

\textit{e) $W^\pm, Z^0$ and the Higgs boson}
The bosonic version of Eq.~\ref{eq:fermionsum} can be used as a first estimate:
\begin{equation}
p/T^4 = \frac{1}{2\pi^2} \sum_i g_i \left(\frac{m_i}{T}\right)^2 \sum_{k=1}^{\infty} \frac{1}{k^2} K_2\left(\frac{mk}{T}\right)\,.
\end{equation}
Refs.~\cite{Laine:2006cp} goes beyond this and adds the one-loop electroweak corrections.
The one loop corrections become noticeable at the
temperature of approximately $T\gtrsim 90~\mathrm{GeV}$. For this correction
we use the data of Refs.~\cite{Laine:2006cp}.

\textit{f) The electroweak transition}
For the electroweak epoch  we quote the results of Laine and Meyer
\cite{Laine:2015kra}. They use perturbation theory, dimensional reduction and
the results of 3D simulations to estimate the equation of state of the Standard
Model near the electroweak transition.  This is a continuation of the earlier
work \cite{Laine:2006cp}.  Although at the time continuum extrapolated
electroweak lattice input was not yet available \cite{Onofrio:2014kta}, the
final continuum extrapolation shows a very mild lattice spacing dependence
\cite{Onofrio:2015mpa}. 
%It is a well known fact, that perturbation theory converges rather slowly,
%however, once we demonstrated the convergence, we can use the perturbative
%results in Ref. \cite{Laine:2015kra}

%Having nonperturbative QCD data up to 1 GeV we have seen that the $g^5$ order
%gives a remarkably good description, already. Since Ref.~\cite{Laine:2015kra}
%have similar assumption on the convergence of the perturbative series
%as Ref.~\cite{Laine:2006cp} we modify the electroweak equation of state
%of Ref.~\cite{Laine:2015kra} such that it is based on the five flavor
%massless $g^5$ order perturbative QCD result.

Adding all components from a) to f) we arrive at the our final result for 
$g(T)$ and $h(T)$ that we show in the main text.


%\begin{figure}[ht]
%\begin{center}
%\centerline{
%\includegraphics[width=2.5in]{comp_g}
%\includegraphics[width=2.5in]{comp_h}
%}
%\includegraphics[width=3in,angle=270]{fig:fullgh}
%\end{center}
%\caption{
%\label{fig:fullgh}
%The QCD contribution to the number of effective degree of freedom $g(T)$
%from our lattice data, continued with the $g^6$ order perturbative result.
%The earlier estimate \cite{Laine:2006cp} is shown for comparison.
%}
%\end{figure}
%


\begin{table}
\begin{center}
\begin{tabular}{|c|c|c|}
\hline
$\log_{10} T/\mathrm{MeV}$&$g_\rho(T)$ & $g_\rho(T)/g_s(T)$\\
\hline
0.00 & 10.71 & 1.00237\\
0.50 & 10.74 & 1.00022\\
1.00 & 10.76 & 1.00043\\
1.25 & 11.09 & 1.00485\\
1.50 & 12.83 & 1.01908\\
2.00 & 17.59 & 1.02308\\
2.10 & 20.36 & 1.03863\\
2.20 & 29.52 & 1.07853\\
2.30 & 40.72 & 1.07966\\
2.40 & 47.76 & 1.06117\\
2.50 & 52.90 & 1.04732\\
3.00 & 73.49 & 1.01769\\
4.00 & 83.11 & 1.00122\\
4.30 & 85.54 & 1.00394\\
4.60 & 92.00 & 1.00874\\
5.00 & 102.15 & 1.00774\\
5.40 & 104.91 & 1.00122\\
5.60 & 104.60 & 1.0000\\
\hline
\end{tabular}
\end{center}
\caption{\label{tab:spline}
Data set on the logarithmic scale that can be used with simple cubic spline interpolation
to find a parametrization on for the entire Standard Model. 
The spline's typical deviation from $g_\rho$ is about 1\%, and 0.3\% for the ratio.
}
\end{table}
